# Supplementary material for: Global Memory from Local Hysteresis in an Amorphous Solid
Source: arXiv:1809.08505 source file (2020-01-27)
Supplement: Supplementary file 1 [file suppmat.pdf]

# Supplemental Materials for "Global Memory from Local Hysteresis in an Amorphous Solid"

Nathan C. Keim, Jacob Hass, Brian Kroger, and Devin Wieker

**Area fraction** — We estimate area fraction using ImageJ. We apply a short-pass filter to the image with a cutoff of 200 pixels, to remove large-scale variations in illumination intensity. We then use an image histogram to identify a threshold midway between light and dark values, apply the threshold, fill holes (to remove the bright optical artifact at the center of large particles), and count the fraction of pixels that represent particles, obtaining an area fraction of 0.36. To estimate uncertainty, we repeat this procedure using a range of threshold values that (roughly speaking) do not make many small particles disappear or allow many nearby particles to be merged. This variation results in an uncertainty of $\pm 0.04$.

**Readout curves** — We perform 6 trials for each training protocol represented in Fig. 1 of the main paper. The readout curves are averages after discarding 0–2 outliers from each set that were contaminated by large spontaneous rearrangements, perhaps from external vibrations, or from interactions among rearranging clusters that led to irreversible changes (see discussion in main text). The complete set of curves that were averaged to make the readout plots of Figs. 1c and 3b in the paper is shown here in Fig. 1, with outliers plotted

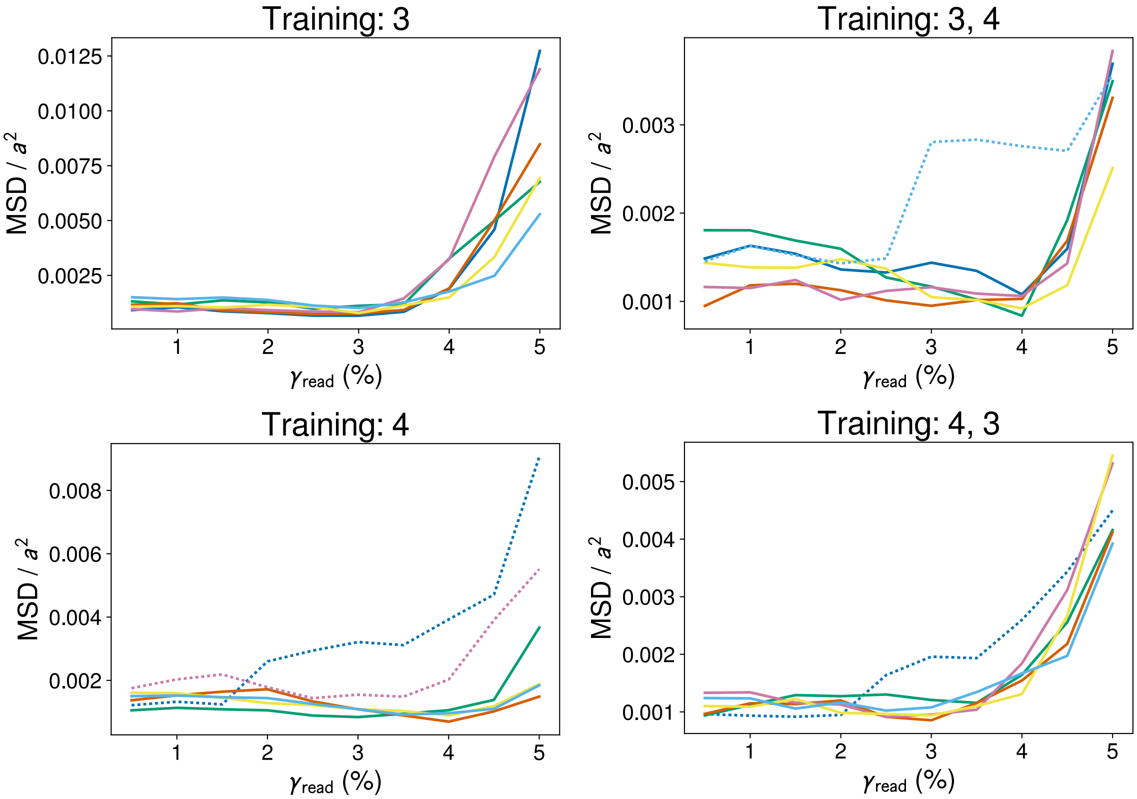


FIG. 1: Readout curves from all trials, averaged to make Figs. 1c and 2b in the main paper, for each training protocol. Outliers that were discarded are plotted as dashed lines.

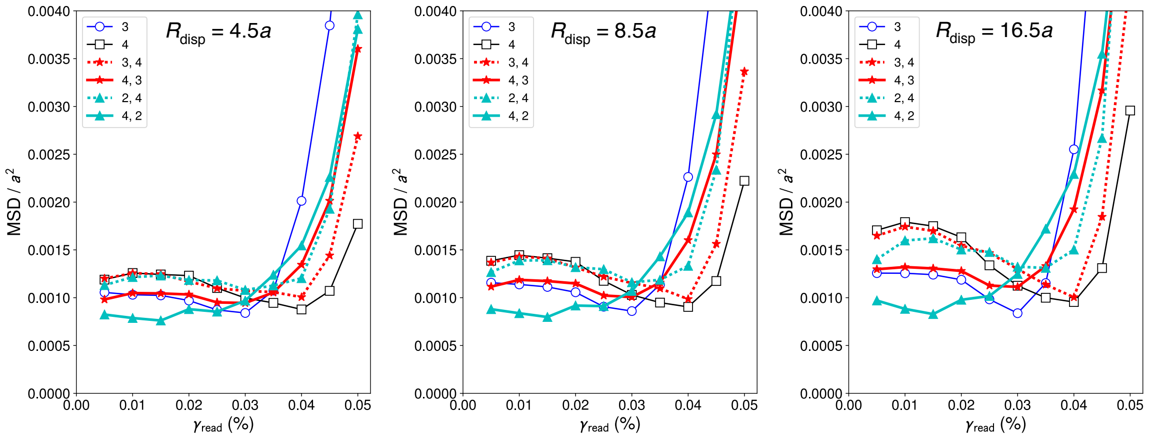


FIG. 2: Effect of varying the radius $R_{\rm disp}$ used to subtract the average motion of nearby particles, when computing $\vec{r}_{\rm local}$. The middle plot is the value used for all other analyses, here and in the main paper. These plots also include results from the "2, 4" and "4, 2" training protocols, that for simplicity were not shown in the main paper, but that are consistent with other results.

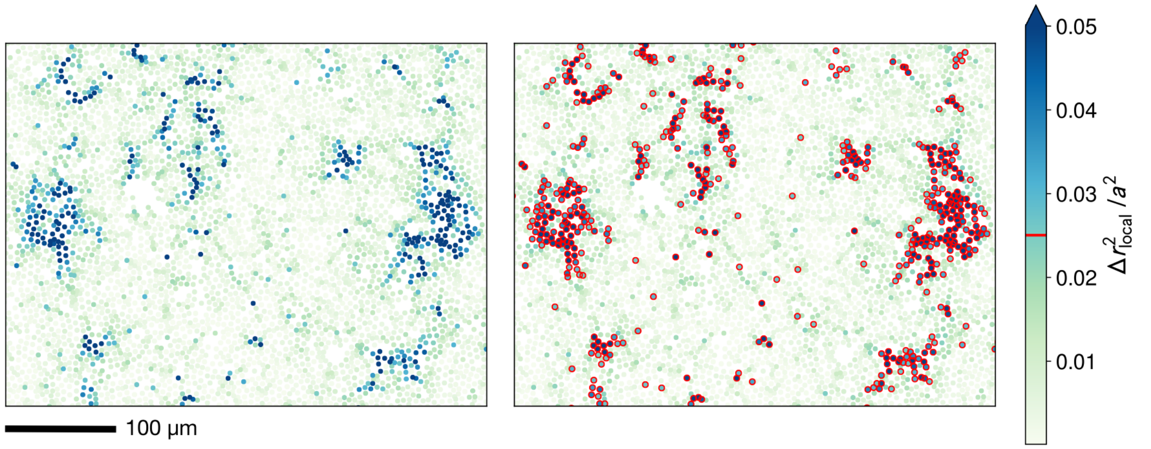


FIG. 3: Particles and $r^2_{\rm local}$ values considered to identify rearranging clusters shown in Fig. 1a of the main paper, for the analysis in Fig. 5 of main paper. Color shows maximum observed $\Delta r^2_{\rm local}/a^2$ of each particle during the interval in Fig. 5a of main paper, as sampled whenever $\gamma = 0$ (twice per cycle). The right panel is identical except for red circles that highlight particles that met the threshold value of 0.025.

as dashed lines. Note that like the other trials, each outlier has a non-monotonic dip that permits an approximate readout of memory.

**Choice of $R_{\rm disp}$** — To compute $\Delta\vec{r}_{\rm local}$ we subtract the motion of nearby particles within a radius $R_{\rm disp} = 8.5a$, using the "local displacement" algorithm in the software package *philatracks* [1]. Figure 2 shows that changing this value has no qualitative effect on our readout results.

**Threshold to identify rearranging clusters** — To identify rearranging particles

shown in Fig. 1a of the main text, for the analysis in Fig. 5 of the main text, we apply a threshold in $\Delta r^2_{\mathrm{local}}/a^2$. Figure 3 shows the application of this threshold, for the region of material shown in Fig. 1a of the main text. To produce Fig. 1a in the main text, we ignore isolated particles that meet the threshold but have no rearranging neighbors (i.e. clusters of size 1).

While the exact outlines of each cluster are sensitive to our choice of threshold, significant clusters (such as the ones we analyze) are separated by regions with much lower values of $\Delta r^2_{\mathrm{local}}/a^2$ than our threshold. A possible exception is the large cluster on the right side, labeled "E" in Fig. 1a of the main text, which can be split into two or more sub-clusters with a modest increase in threshold to $\sim 0.04$. We find that in this case, the two smaller clusters both have the same behavior as the original does in the analysis of Fig. 5c in the main paper.

[1] N. C. Keim, *Philatracks v0.2*, DOI:10.5281/zenodo.11459 (2014), URL `https://github.com/nkeim/philatracks`.
